# Supplementary material for: Radium-containing molecular cations amenable for laser cooling
Source: arXiv:2205.14429 ancillary file (2022-05-28)
Supplement: Supplementary file 1 [file Supplementary-1.pdf]

# Supplementary materials for MS “ Radium-containing molecular cations amenable for laser cooling”

TABLE I. Exponential parameters  $\zeta$  for diffuse and polarization functions used in RDFT calculations

| Atom | <i>s</i> | <i>p</i> | <i>d</i> | <i>f</i> |
|------|----------|----------|----------|----------|
| H    |          | 1.40700  |          |          |
|      |          | 0.38800  |          |          |
| C    | 0.04690  | 0.04041  | 0.55000  |          |
|      |          |          | 0.15100  |          |
| N    | 0.06124  | 0.05611  | 0.81700  |          |
|      |          |          | 0.23000  |          |
| F    | 0.09863  | 0.08502  | 1.64000  |          |
|      |          |          | 0.46400  |          |
| Ra   |          |          |          | 1.13910  |
|      |          |          |          | 0.41836  |
|      |          |          |          | 0.15633  |
|      |          |          |          | 0.07074  |

Data (in Wolfram Mathematica format) for PEC of the ground and excited electronic states of RaNCH<sup>+</sup> cation

```
X_state = {{4.843280, -0.023436593}, {5.043280, -0.028156902}, {5.243280, -0.03054522},
{5.44328, -0.031360168}, {5.64328, -0.031146861}, {5.84328, -0.030291099},
{6.043280, -0.029060911}}
1_state = {{4.843280, 0.023286017}, {5.043280, 0.021662305}, {5.243280, 0.02065368},
```

```

{5.44328, 0.02040203}, {5.64328, 0.02094465}, {5.84328, 0.02207783},
{6.043280, 0.02358168}}
2_state = {{4.843280, 0.021910461}, {5.043280, 0.02097725}, {5.243280, 0.02117916},
{5.44328, 0.02211756}, {5.64328, 0.02352677}, {5.84328, 0.02521443},
{6.043280, 0.02703757}}
3_state = {{4.843280, 0.031106089}, {5.043280, 0.02697303}, {5.243280, 0.02588777},
{5.44328, 0.026501641}, {5.64328, 0.027920662}, {5.84328, 0.029734139},
{6.043280, 0.031724471}}
4_state = {J=5/2 - no transitions!}
5_state = {{4.843280, 0.052075356}, {5.043280, 0.046597802}, {5.243280, 0.043513249},
{5.44328, 0.042002275}, {5.64328, 0.041502296}, {5.84328, 0.041636239},
{6.043280, 0.042153517}}

```
